# Supplementary material for: Self-Calibrating Neural Radiance Fields
Source: arXiv:2108.13826 source file (2021-09-02)
Supplement: Supplementary file 1 [file llff.tex]

\section{NeRF-LLFF Experiments}

We also conduct more experiments on the NeRF-LLFF dataset. We train intrinsic parameters, extrinsic parameters, and non-linear distortion parameters. Table~\ref{tab:supp_llff_test} shows the rendering quality on the test set. Table~\ref{tab:supp_llff_train} shows the rendering quality and the projected ray distance loss on the train set. For "leaves" scene, we do not report the ray distance since we found that the correspondences from SuperGlue~\cite{wang2019superglue} were inaccurate, which led to high projected ray distance above the threshold $\eta$.

\begin{table*}[h]
\centering
\caption{Experiment on the NeRF-LLFF test set. I + ($N\%$) indicates $N\%$ additive noise on the initial focal length. T $[-\alpha, \alpha]$ indicates additive translation noise between $[-\alpha, \alpha]$. R $[-\theta, \theta]$ indicates additive rotation noise between $[-\theta, \theta]$. T $[-\alpha, \alpha]$ + R $[-\theta, \theta]$ indicates both random rotation noise between $[-\theta, \theta]$ and random translation noise between $[-\alpha, \alpha]$. \label{tab:supp_llff_test}}
\resizebox{\textwidth}{!}{
\begin{tabular}{|c|c|c|c|c|} 
\hline
\multirow{2}{*}{PSNR($\uparrow$) / SSIM($\uparrow$) / LPIPS($\downarrow$)}                                          & \multicolumn{2}{c|}{Room}                                                & \multicolumn{2}{c|}{Leaves}                  \\ 
\cline{2-5}
                                                                              & NeRF                       & ours                      & NeRF                                         & ours                       \\
\hline
I (+ 1\%)                                                                     & 22.286 / 0.8003 / 0.1485   & \textbf{32.986 / 0.9581 / 0.1069}  &   16.389 / 0.4518 / 0.2745                   & \textbf{22.643 / 0.8113 / 0.1843}   \\
\hline
I (+ 2\%)                                                                     & 19.315 / 0.7081 / 0.1978   & \textbf{33.027 / 0.9586 / 0.1082}  &   14.145 / 0.2366 / 0.3472                   & \textbf{22.684 / 0.8125 / 0.1862}   \\
\hline
I (+ 5\%)                                                                     & 16.624 / 0.6105 / 0.3036   & \textbf{32.941 / 0.9576 / 0.1089}  &   12.341 / 0.1283 / 0.4700                   & \textbf{22.687 / 0.8130 / 0.1864}   \\
\hline
I (+10\%)                                                                     & 15.573 / 0.5528 / 0.4111   & \textbf{32.870 / 0.9583 / 0.1078}  &   11.329 / 0.0912 / 0.5610                   & \textbf{22.706 / 0.8156 / 0.1855}   \\
\hline
I (+20\%)                                                                     & 14.687 / 0.4871 / 0.5214   & \textbf{33.061 / 0.9583 / 0.1051}  &   10.789 / 0.0770 / 0.6375                   & \textbf{22.742 / 0.8162 / 0.1869}   \\
\hline
T ( [-0.01, 0.01] )                                                           & 26.458 / 0.8924 / 0.2221   & \textbf{26.820 / 0.8966 / 0.2199}  &   21.678 / 0.7599 / 0.2488                   & \textbf{21.817 / 0.7720 / 0.2262}   \\
\hline
T ( [-0.02, 0.02] )                                                           & 22.895 / 0.7909 / 0.3372   & \textbf{23.240 / 0.8137 / 0.3190}  &   20.363 / 0.6811 / 0.3153                   & \textbf{20.593 / 0.7027 / 0.2870 }  \\
\hline
T ( [-0.05, 0.05] )                                                           & 19.208 / 0.6294 / 0.4900   & \textbf{19.993 / 0.6822 / 0.4574}  &   17.430 / 0.4736 / 0.4564                   & \textbf{17.884 / 0.5236 / 0.4061}   \\
\hline
R ( [-0.5, 0.5] )                                                             & 23.501 / 0.7881 / 0.3513   & \textbf{23.768 / 0.8025 / 0.3363}  &   \textbf{17.447} / 0.4450 / 0.4738          & 17.352 / \textbf{0.4462 / 0.4527}   \\
\hline
R ( [-1.0, 1.0] )                                                             & 20.631 / 0.6809 / 0.4573   & \textbf{21.063 / 0.7038 / 0.4445}  &   15.089 / 0.2364 / 0.5898                   & \textbf{15.221 / 0.2638 / 0.5546}   \\
\hline
R ( [-5.0, 5.0] )                                                             & 15.377 / 0.4153 / 0.6496   & \textbf{16.866 / 0.4793 / 0.6008}  &   11.361 / 0.0798 / 0.6853                   & \textbf{11.847 / 0.0843 / 0.6400}   \\
\hline
\begin{tabular}[c]{@{}c@{}}T ([-0.01, 0.01])\\+ R ([-0.5, 0.5]) \end{tabular} & 22.643 / 0.7590 / 0.3751   & \textbf{22.872 / 0.7765 / 0.3601}  &   \textbf{17.009} / 0.4042 / 0.5013          & 16.960 / \textbf{0.4109 / 0.4747}   \\
\hline
\begin{tabular}[c]{@{}c@{}}T ([-0.02, 0.02])\\+ R ([-1.0, 1.0]) \end{tabular} & 20.029 / 0.6469 / 0.4773   & \textbf{20.307 / 0.6796 / 0.4572}  &   14.661 / 0.2000 / 0.6054                   & \textbf{14.699 / 0.2089 / 0.5751}   \\
\hline
\begin{tabular}[c]{@{}c@{}}T ([-0.05, 0.05])\\+ R ([-5.0, 5.0]) \end{tabular} & 14.979 / 0.3882 / 0.6578   & \textbf{16.609 / 0.4483 / 0.6099}  &   11.309 / 0.0766 / 0.6868                   & \textbf{11.638 / 0.0766 / 0.6453 }  \\
\hline
\end{tabular}
}
\end{table*}

\begin{table*}[h]
\centering
\caption{Experiment on the NeRF-LLFF train set. I + ($N\%$) is the experiment that adds $N\%$ noise in the initial focal length. T $[-\alpha, \alpha]$ is the experiment that adds random translation noise between $[-\alpha, \alpha]$ in initial camera extrinsic parameters. R $[-\theta, \theta]$ is the experiment that adds random rotation noise between $[-\theta, \theta]$ in initial extrinsic parameters. T $[-\alpha, \alpha]$ + R $[-\theta, \theta]$ is the experiment that adds both random rotation noise between $[-\theta, \theta]$ and random translation noise between $[-\alpha, \alpha]$. For leaves scene, we do not report ray distances in some experiments since no correct correspondences were found with noisy camera parameters. \label{tab:supp_llff_train}}
\resizebox{\textwidth}{!}{
\begin{tabular}{|c|c|c|c|c|} 
\hline
\multirow{2}{*}{PSNR($\uparrow$) / SSIM($\uparrow$) / LPIPS($\downarrow$)}                                          & \multicolumn{2}{c|}{Room}                                                & \multicolumn{2}{c|}{Leaves}                  \\ 
\cline{2-5}
                                                                                    & NeRF                                & ours                                & NeRF                                         & ours                               \\
\hline
I (+ 1\%)                                                                           & \textbf{37.418 / 0.9736 / 0.0871} / 2.5327   & 36.939 / 0.9714 / 0.0900 / \textbf{0.2926}   & 24.182 / 0.8457 / 0.1753 / -                  & \textbf{24.732 / 0.8596 / 0.1597} / 0.4114   \\
\hline
I (+ 2\%)                                                                           & \textbf{37.269 / 0.9727 / 0.08967} / 2.4986  & 36.924 / 0.8712 / 0.0919 / \textbf{0.2919}   & 24.052 / 0.8422 / 0.1767 / -                  & \textbf{24.728 / 0.8596 / 0.1588} / 0.4232   \\
\hline
I (+ 5\%)                                                                           & 36.694 / 0.9706 / 0.09497 / 2.4245  & \textbf{36.915 / 0.9710 / 0.0935 / 0.2896}   & 23.182 / 0.8127 / 0.2050 / 2.6422             & \textbf{24.709 / 0.8587 / 0.1601 / 0.4189}   \\
\hline
I (+10\%)                                                                           & 35.205 / 0.9637 / 0.1104 / 2.7394   & \textbf{36.902 / 0.9714 / 0.0919 / 0.2847}   & 21.698 / 0.7429 / 0.2729 / 2.5665             & \textbf{24.732 / 0.8602 / 0.1604 / 0.4281}   \\
\hline
I (+20\%)                                                                           & 32.786 / 0.9445 / 0.1578 / 2.4648   & \textbf{36.889 / 0.9713 / 0.0911 / 0.2830}   & 19.459 / 0.5936 / 0.3978 / 2.4167             & \textbf{24.723 / 0.8597 / 0.1610 / 0.4478}   \\
\hline
T ( [-0.01, 0.01] )                                                                 & 28.230 / 0.9104 / 0.2140 / 2.5848   & \textbf{30.386 / 0.9190 / 0.2017 / 0.7163}   & 23.016 / 0.8007 / 0.2241 / -                  & \textbf{23.404 / 0.8113 / 0.2042} / 0.6077   \\
\hline
T ( [-0.02, 0.02] )                                                                 & 24.832 / 0.8173 / 0.3508 / 2.6021   & \textbf{28.131 / 0.8696 / 0.2987 / 1.2610}   & 21.418 / 0.7237 / 0.2966 / -                  & \textbf{22.055 / 0.7508 / 0.2683} / 0.8076   \\
\hline
T ( [-0.05, 0.05] )                                                                 & 20.204 / 0.6684 / 0.4854 / 2.5943   & \textbf{26.310 / 0.8023 / 0.4305 / 1.7343}   & 18.295 / 0.5232 / 0.4432 / -                  & \textbf{19.964 / 0.6337 / 0.3822} / 1.1569   \\
\hline
R ( [-0.5, 0.5] )                                                                   & 24.832 / 0.8173 / 0.3508 / 2.5713   & \textbf{27.696 / 0.8617 / 0.3216 / 1.5427}   & 18.304 / 0.4959 / 0.4556 / -                  & \textbf{19.177 / 0.5490 / 0.4276} / 1.7468   \\
\hline
R ( [-1.0, 1.0] )                                                                   & 21.615 / 0.7077 / 0.4594 / 2.6741   & \textbf{26.209 / 0.8095 / 0.4193 / 1.7285}   & 16.006 / 0.2950 / 0.5655 / -                  & \textbf{18.253 / 0.4673 / 0.5135} / 1.8232   \\
\hline
R ( [-5.0, 5.0] )                                                                   & 16.423 / 0.4751 / 0.6416 / 2.7014   & \textbf{24.491 / 0.6858 / 0.5673 / 1.7273}   & 12.543 / 0.1322 / 0.6592 / -                  & \textbf{17.738 / 0.4362 / 0.5702} / 1.4266   \\
\hline
\begin{tabular}[c]{@{}c@{}}T ([-0.01, 0.01])\\+ R ([-0.5, 0.5]) \end{tabular}       & 24.145 / 0.7976 / 0.3701 / 2.5699   & \textbf{27.404 / 0.8530 / 0.3424 / 1.5853}   & 17.944 / 0.4634 / 0.4778 / -                  & \textbf{19.042 / 0.5349 / 0.4432} / 1.7532   \\
\hline
\begin{tabular}[c]{@{}c@{}}T ([-0.02, 0.02])\\+ R ([-1.0, 1.0]) \end{tabular}       & 21.071 / 0.6861 / 0.4767 / 2.6424   & \textbf{26.047 / 0.8016 / 0.4312 / 1.7622}   & 15.491 / 0.2536 / 0.5863 / -                  & \textbf{18.135 / 0.4558 / 0.5268} / 1.7275   \\
\hline
\begin{tabular}[c]{@{}c@{}}T ([-0.05, 0.05])\\+ R ([-5.0, 5.0]) \end{tabular}       & 16.193 / 0.4354 / 0.6593 / 2.7682   & \textbf{24.779 / 0.6850 / 0.5692 / 1.7464}   & 12.133 / 0.1094 / 0.6752 / -                  & \textbf{17.857 / 0.4449 / 0.5684} / 1.4624   \\
\hline
\end{tabular}
}
\end{table*}
